# Supplementary material for: Enhancing End-to-End Autonomous Driving with Risk Semantic Distillaion from VLM
Source: arXiv:2511.14499 source file (2025-11-18)
Supplement: Supplementary file 1 [file X_suppl.tex]

%%%%%%%%%%%%%%%%%%%%%%%%%%%%%%%%%%%%%%%%%%%%%%%%%%%%%%%%%%%%

\appendix
\newpage

% % \clearpage
% % \setcounter{page}{1}
% % \maketitlesupplementary
% % \newpage

% \clearpage
% % \maketitlesupplementary
% \appendix
% \onecolumn
% \setcounter{page}{1}
\section*{Appendix}
% \appendix
\section{Method}
\subsection{Risk Semantic Annotaion}
\label{Appendix: Risk Semantic Annotaion}
TASKDISCRIPTION = "You are the brain of an autonomous vehicle. These image sequences are returned by your forward-facing camera. Analyze the risk critical objects in the diagram, such as occlusion that vehicles comes to lanes of ego vehicle suddenly or motorcycles obscured by cars or pedestrains obscured by cars, and you must detect all these critical objects in the image with its bounding box. And you can use the information from another grounding model, which describe the location of different objects. Notice that the socre of json is the confidence score of bbox."

STATEINFO = 
\begin{verbatim}
{'label':'car',
'points':
[[356.63262939453125,1010.9845581054688],
[1474.0504150390625,1619.9420166015625]],
'group_id': null,
'shape_type': 'rectangle',
'description': 'score: 0.735',
'flags': {}}
\end{verbatim}

OUTPUTFORMAT = "You must output the object in a risk order and don't omit the isntance with bbox in the image, and don't output any text other than the json data. Please note that if a median or fence is observed between a neighboring vehicle and your own vehicle, this should not be considered a risk. Please note that if you think the risk level of an object is high, its risk score should not be lower than 0.7; if you think the risk of an object is low, its risk score should not be higher than 0.3; and for the object in a medium risk level, its score should be between 0.3-0.7; Be careful not to pay too much risk attention to oncoming vehicles. You must output information in the json format followed and give rank based on the risk level, 
\begin{verbatim}
{      
    '0':{ 
    'category_id':1,
    'bbox':[126, 87, 398, 444],
    'risk_score':0.93,
    'risk_level': 'high'
    'category_name':'bus', 
    'reason':'the bus is very close to the ego vehicle' 
    }, 
    '1': { 
    'category_id': 3,  
    'bbox': [299,325,412,393], 
    'risk_score': 0.21, 
    'risk_level': 'low', 
    'category_name': 'car', 
    'reason': 
    'the car is parked along the road'} 
    '2': { 
    'category_id': 3,  
    'bbox': [199,325,432,383], 
    'risk_score': 0.41, 
    'risk_level': 'mediam', 
    'category_name': 'car', 
    'reason': 'The vehicle is in the opposite lane'},
}"
\end{verbatim}    

\label{sec:rationale}
Having the supplementary compiled together with the main paper means that:
\begin{itemize}
\item The supplementary can back-reference sections of the main paper, for example, we can refer to \ref{sec:intro};
\item The main paper can forward reference sub-sections within the supplementary explicitly (e.g. referring to a particular experiment); 
\item When submitted to arXiv, the supplementary will already included at the end of the paper.
\end{itemize}

\subsection{BEV Rebatching Procedure}
\label{BEV Rebatching Procedure}
In multi-view perception systems, it is computationally inefficient to allow all camera views to attend to all Bird's Eye View (BEV) queries\cite{vaswani2017attention}. For BEV feature, we must have a special BEV mask and rebatch process, that is, for a BEV feature, the projected 2D point can only fall on some of the six PV views, while the other views are not hit. Here, we call the hit view $V_{hit}$\cite{li2024bevformer}. To improve memory efficiency and inference speed, we introduce a rebatching procedure\cite{li2024bevformer} in which each camera only processes those BEV queries that are within its field of view. The details can be found in Appendix.~\ref{BEV Rebatching Procedure}.

This is accomplished by constructing a \textbf{BEV visibility mask}, denoted as $\text{BEV\_mask}$, which identifies which BEV queries are visible from which cameras. The BEV visibility mask is generated by projecting a set of reference 3D points, sampled from elevated BEV queries, into 2D camera image planes using the \texttt{lidar2img} transformation matrices. The transformation pipeline can be expressed as follows. Each normalized reference point $r_i = (x, y, z)$ in the BEV volume is first scaled by the point cloud range $(x_{\min}, x_{\max}, y_{\min}, y_{\max}, z_{\min}, z_{\max})$:
\begin{equation}
r_i^{\text{scaled}} = 
\begin{bmatrix}
x \cdot (x_{\max} - x_{\min}) + x_{\min} \\
y \cdot (y_{\max} - y_{\min}) + y_{\min} \\
z \cdot (z_{\max} - z_{\min}) + z_{\min} \\
1
\end{bmatrix}
\in \mathbb{R}^{4}
\end{equation}

Each point is then transformed into the 2D image space using the camera projection matrix:$
r_i^{\text{cam}} = \text{lidar2img}_k \cdot r_i^{\text{scaled}}, \quad k = 1, \dots, N_{\text{cam}}.$ The resulting 2D pixel coordinates are obtained by:
\(
(x_{\text{2D}}, y_{\text{2D}}) = \left( \frac{r_i^{\text{cam}}[0]}{r_i^{\text{cam}}[2]}, \frac{r_i^{\text{cam}}[1]}{r_i^{\text{cam}}[2]} \right)
\). These coordinates are normalized by the image dimensions $(W, H)$:
\(
x_{\text{norm}} = \frac{x_{\text{2D}}}{W}, \quad y_{\text{norm}} = \frac{y_{\text{2D}}}{H}
\). 
A BEV query is considered visible in camera $k$ if:
\begin{equation}
\text{BEV\_mask}_{k, i} = 
\begin{cases}
1 & \text{if } 0 < x_{\text{norm}} < 1 \text{ and } 0 < y_{\text{norm}} < 1 \text{ and } r_i^{\text{cam}}[2] > \epsilon \\
0 & \text{otherwise}
\end{cases}
\end{equation}
Let $\mathcal{BEV} \in \mathbb{R}^{B \times N_{BEV} \times d}$ denote the original BEV query tensor, and let $\mathcal{R}_{2d} \in \mathbb{R}^{ B  \times N_{\text{cam}} \times N_{BEV} \times D \times 2}$ be the projected 2D reference points. We first extract the set of valid BEV queries for each camera:
\begin{equation}
    \mathcal{I}_{k}^{(b)} = \left\{ q \mid \sum_{d=1}^{D} \text{BEV\_mask}_{k}^{(b)}[q, d] > 0 \right\}
\end{equation}
Where q denotes the position of BEV\_mask.
Let $L_{\max} = \max_{k, b} |\mathcal{I}_{k}^{(b)}|$ be the maximum number of visible queries across all views and batches. We initialize rebatching tensors:
\(
\mathcal{BEV}' \in \mathbb{R}^{B \times N_{\text{cam}} \times L_{\max} \times d}, \quad
\mathcal{R}'_{2d} \in \mathbb{R}^{B \times N_{\text{cam}} \times L_{\max} \times D \times 2}
\). For each batch $b$ and camera $k$, we insert the visible queries $q_{vis}$:
\begin{equation}
    \begin{aligned}
        \mathcal{BEV}'[b, k, l] = \mathcal{BEV}&[b, q_{vis}], \quad
        \mathcal{R}'_{2d}[b, k, l, d] = \mathcal{R}_{2d}[d, b, q_{vis}, k]\\
        &\forall q_{vis} \in \mathcal{I}_{k}^{(b)}, \quad l = \text{index}(q_{vis})
    \end{aligned}
\end{equation}

\section{Metrics}
\label{Appendix:Metrics}
\subsection{Perception Metrics}
\label{Perception Metrics}
\paragraph{mAP (mean Average Precision)} 
\[
\text{mAP} = \frac{1}{N} \sum_{i=1}^{N} \text{AP}_i
\]
where \(N\) is the number of categories, and \(\text{AP}_i\) is the Average Precision for the \(i\)-th category. Average Precision is the mean of precision at different recall levels.

\paragraph{mATE (mean Absolute Trajectory Error)} 
\[
\text{mATE} = \frac{1}{T} \sum_{t=1}^{T} \left| \mathbf{p}_t - \hat{\mathbf{p}}_t \right|
\]
where \(T\) is the number of time steps, \(\mathbf{p}_t\) is the true position at time step \(t\), and \(\hat{\mathbf{p}}_t\) is the predicted position at time step \(t\).

\paragraph{mASE (mean Absolute Spatial Error)}
\[
\text{mASE} = \frac{1}{N} \sum_{i=1}^{N} \left| \mathbf{p}_i - \hat{\mathbf{p}}_i \right|
\]
where \(N\) is the number of spatial predictions, \(\mathbf{p}_i\) is the true spatial position, and \(\hat{\mathbf{p}}_i\) is the predicted spatial position.

\paragraph{mAOE (mean Absolute Orientation Error)}
\[
\text{mAOE} = \frac{1}{N} \sum_{i=1}^{N} \left| \theta_i - \hat{\theta}_i \right|
\]
where \(N\) is the number of predicted orientations, \(\theta_i\) is the true orientation at time step \(i\), and \(\hat{\theta}_i\) is the predicted orientation at time step \(i\).

\paragraph{mAVE (mean Absolute Velocity Error)}
\[
\text{mAVE} = \frac{1}{N} \sum_{i=1}^{N} \left| v_i - \hat{v}_i \right|
\]
where \(N\) is the number of predicted velocities, \(v_i\) is the true velocity at time step \(i\), and \(\hat{v}_i\) is the predicted velocity at time step \(i\).

\paragraph{NDS (Normalized Discounted Score)}
\[
\text{NDS} = \frac{1}{M} \sum_{m=1}^{M} \frac{\text{score}_m}{\log_2(m+1)}
\]
where \(M\) is the number of evaluation tasks, \(\text{score}_m\) is the score for the \(m\)-th task, and \(\log_2(m+1)\) is the discount factor for the score.

\subsection{Planning Metrics}
\label{Planning Metrics}
\paragraph{Average Displacement Error (ADE,plan\_L2\_metric)}
The Average Displacement Error (ADE) is a commonly used metric to evaluate the accuracy of predicted trajectories in autonomous systems, such as self-driving vehicles. ADE calculates the average Euclidean distance between the predicted positions and the ground truth positions over a sequence of time steps, providing a quantitative assessment of the prediction quality.

Given a predicted trajectory \( \mathbf{T}_{\text{pred}} = \{(x_i, y_i)\}_{i=1}^{n_{\text{future}}} \) and a corresponding ground truth trajectory \( \mathbf{T}_{\text{gt}} = \{(x_i^{\text{gt}}, y_i^{\text{gt}})\}_{i=1}^{n_{\text{future}}} \), the ADE is defined as the average Euclidean distance between the predicted and ground truth positions across all time steps. Formally, the ADE is computed as:

\[
\text{ADE} = \frac{1}{n_{\text{future}}} \sum_{i=1}^{n_{\text{future}}} \sqrt{(x_i - x_i^{\text{gt}})^2 + (y_i - y_i^{\text{gt}})^2}
\]

Where: \( (x_i, y_i) \) represents the predicted position at time step \( i \), \( (x_i^{\text{gt}}, y_i^{\text{gt}}) \) represents the ground truth position at time step \( i \), \( n_{\text{future}} \) is the total number of time steps over which the trajectory is predicted.

The ADE metric provides a straightforward way to quantify how close the predicted trajectory is to the ground truth. A lower ADE value indicates a better alignment between the predicted and actual trajectories, making it a crucial metric for evaluating trajectory prediction models in real-world applications.

\paragraph{plan\_obj\_box\_col}
The plan\_obj\_box\_col collision indicator is a crucial metric in autonomous driving, as it measures the likelihood of a collision between the ego vehicle and surrounding objects based on the overlap of their bounding boxes. A lower collision probability indicates that the ego vehicle is less likely to collide with objects in its environment, which directly correlates with safer navigation and better trajectory planning. Therefore, a lower value of this metric signifies improved performance of the autonomous system in avoiding obstacles, ensuring smoother and safer driving.

Let \( \mathbf{B}_{\text{car}}(t) \) and \( \mathbf{B}_{\text{obj}}(t) \) represent the bounding boxes of the ego vehicle and the object at time \( t \), respectively. The binary collision indicator \( c_t \) at time \( t \) is defined as:

\[
c_t = \begin{cases} 
1, & \text{if } \mathbf{B}_{\text{car}}(t) \cap \mathbf{B}_{\text{obj}}(t) \neq \emptyset, \\
0, & \text{otherwise}.
\end{cases}
\]

Where \( \mathbf{B}_{\text{car}}(t) \cap \mathbf{B}_{\text{obj}}(t) \) represents the intersection (overlap) between the ego vehicle's bounding box and the object's bounding box at time \( t \). If there is an intersection (overlap), then \( c_t = 1 \), indicating a collision at time \( t \). If there is no intersection, then \( c_t = 0 \), indicating no collision at time \( t \).

The average collision probability over the future \( n_{\text{future}} \) time steps is given by:

\[
\text{plan\_obj\_box\_coll} = \frac{1}{n_{\text{future}}} \sum_{t=1}^{n_{\text{future}}} c_t
\]

Where \( c_t \) is the binary collision indicator for each time step.
 \( n_{\text{future}} \) is the total number of time steps in the prediction window (for example, over 1 second).

\subsection{Bbox-RSD}
\label{Bbox-RSD}
\begin{figure*}[htbp]
    \centering
    % 左侧的单独大图
    \begin{minipage}{0.35\textwidth}
        \centering
        \includegraphics[height=2.7cm]{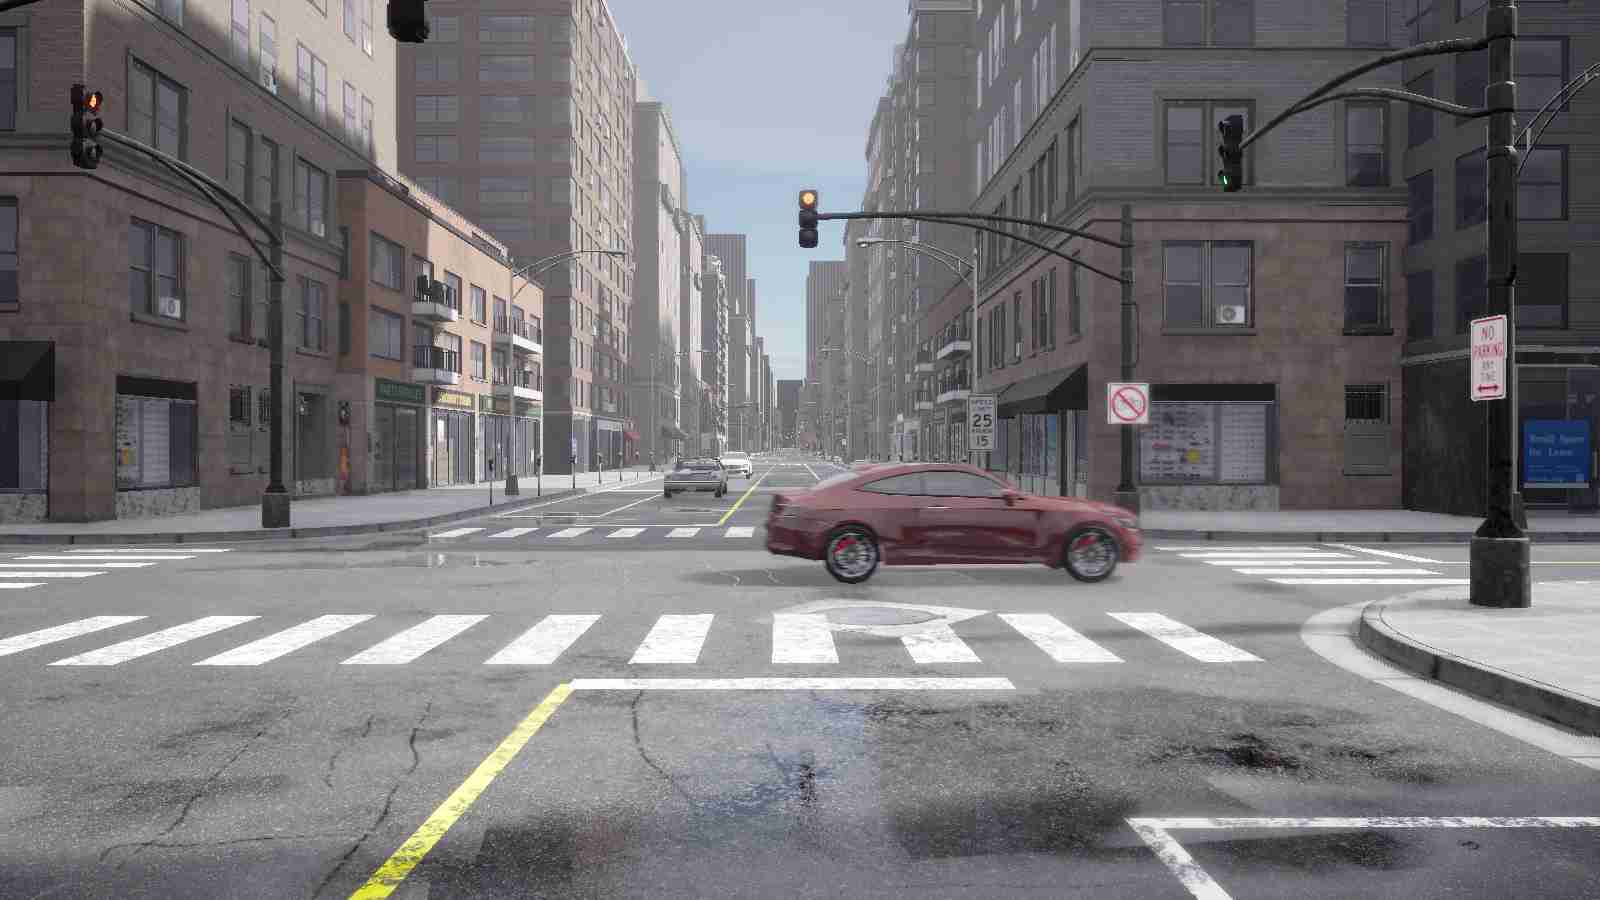}
    \end{minipage}
    \begin{minipage}{0.35\textwidth}
        \centering
        \includegraphics[height=2.7cm]{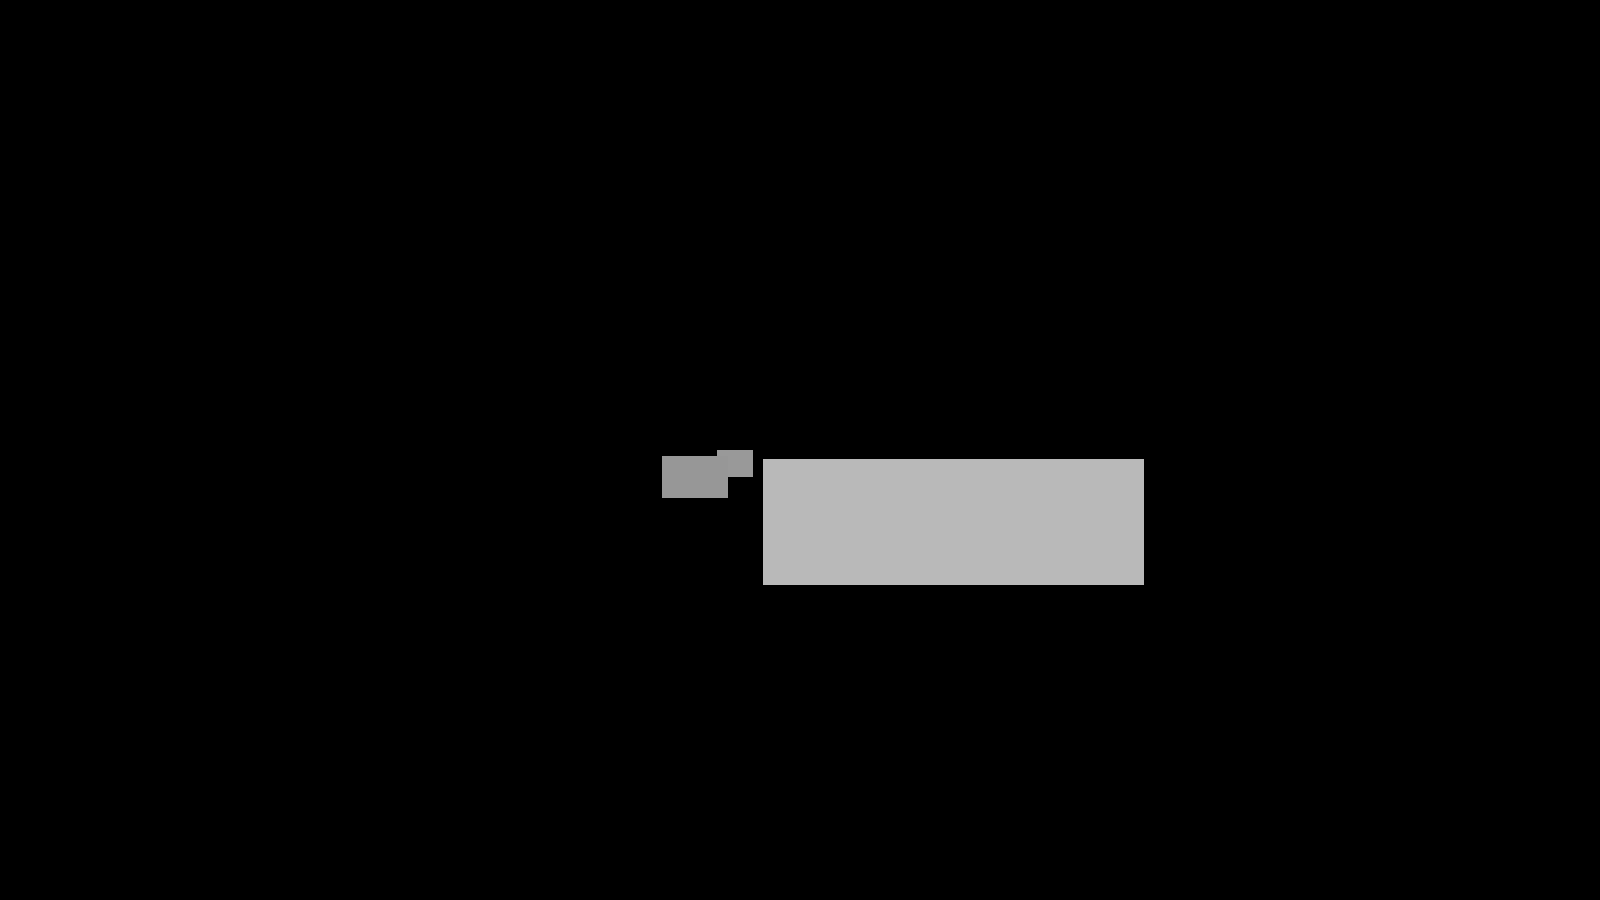}
    \end{minipage}
    \begin{minipage}{0.35\textwidth}
        \centering
        \includegraphics[height=2.7cm]{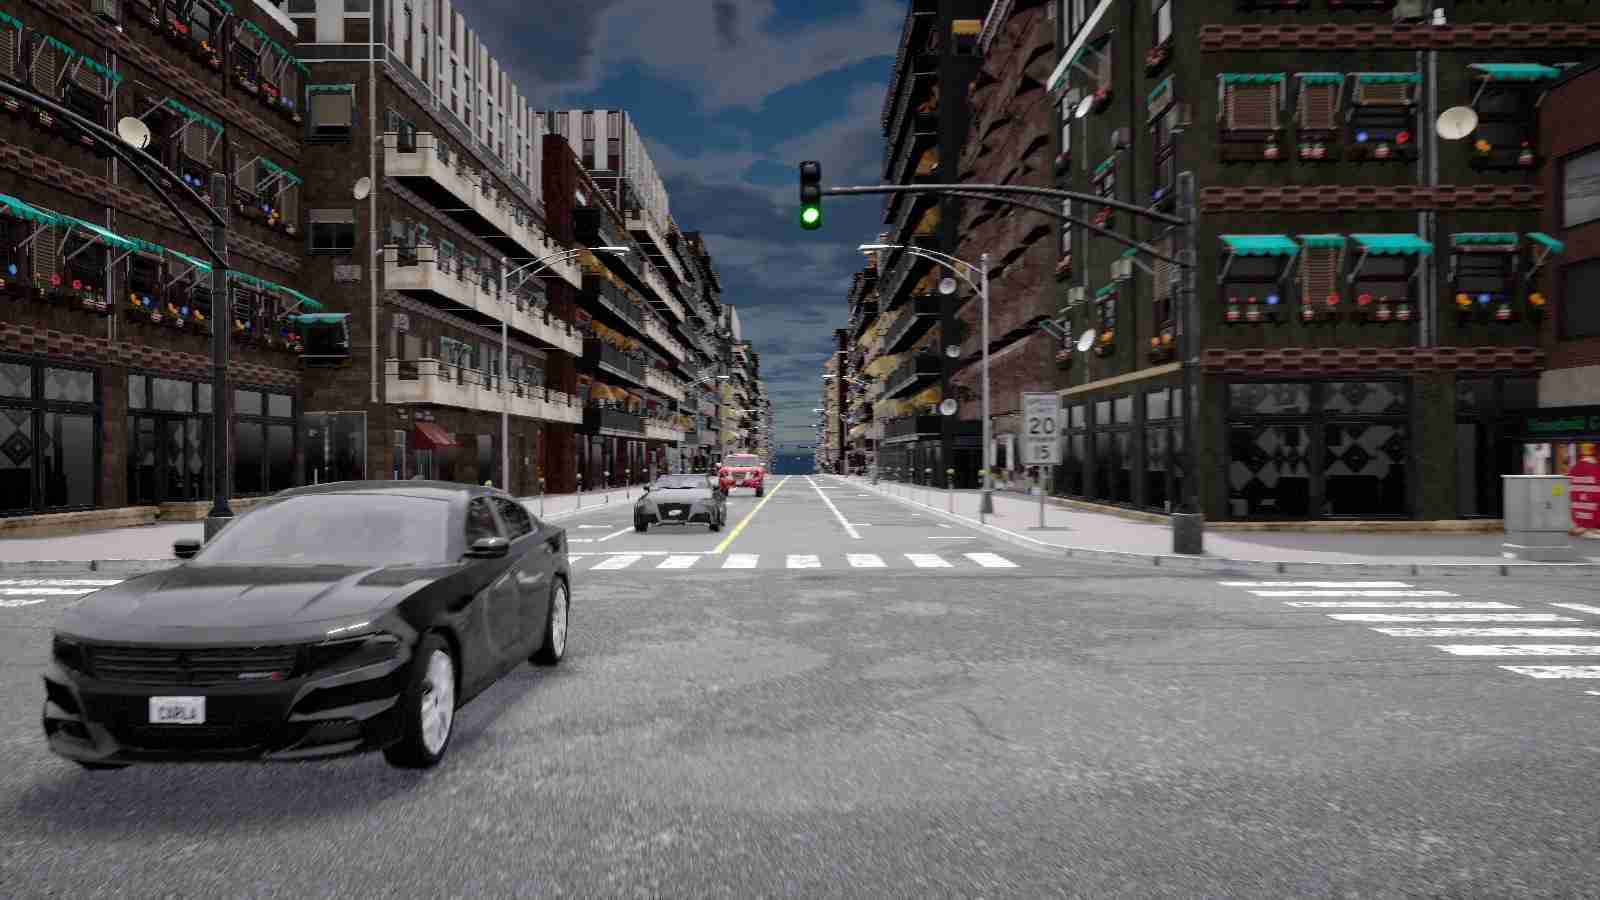}
    \end{minipage}
    \begin{minipage}{0.35\textwidth}
        \centering
        \includegraphics[height=2.7cm]{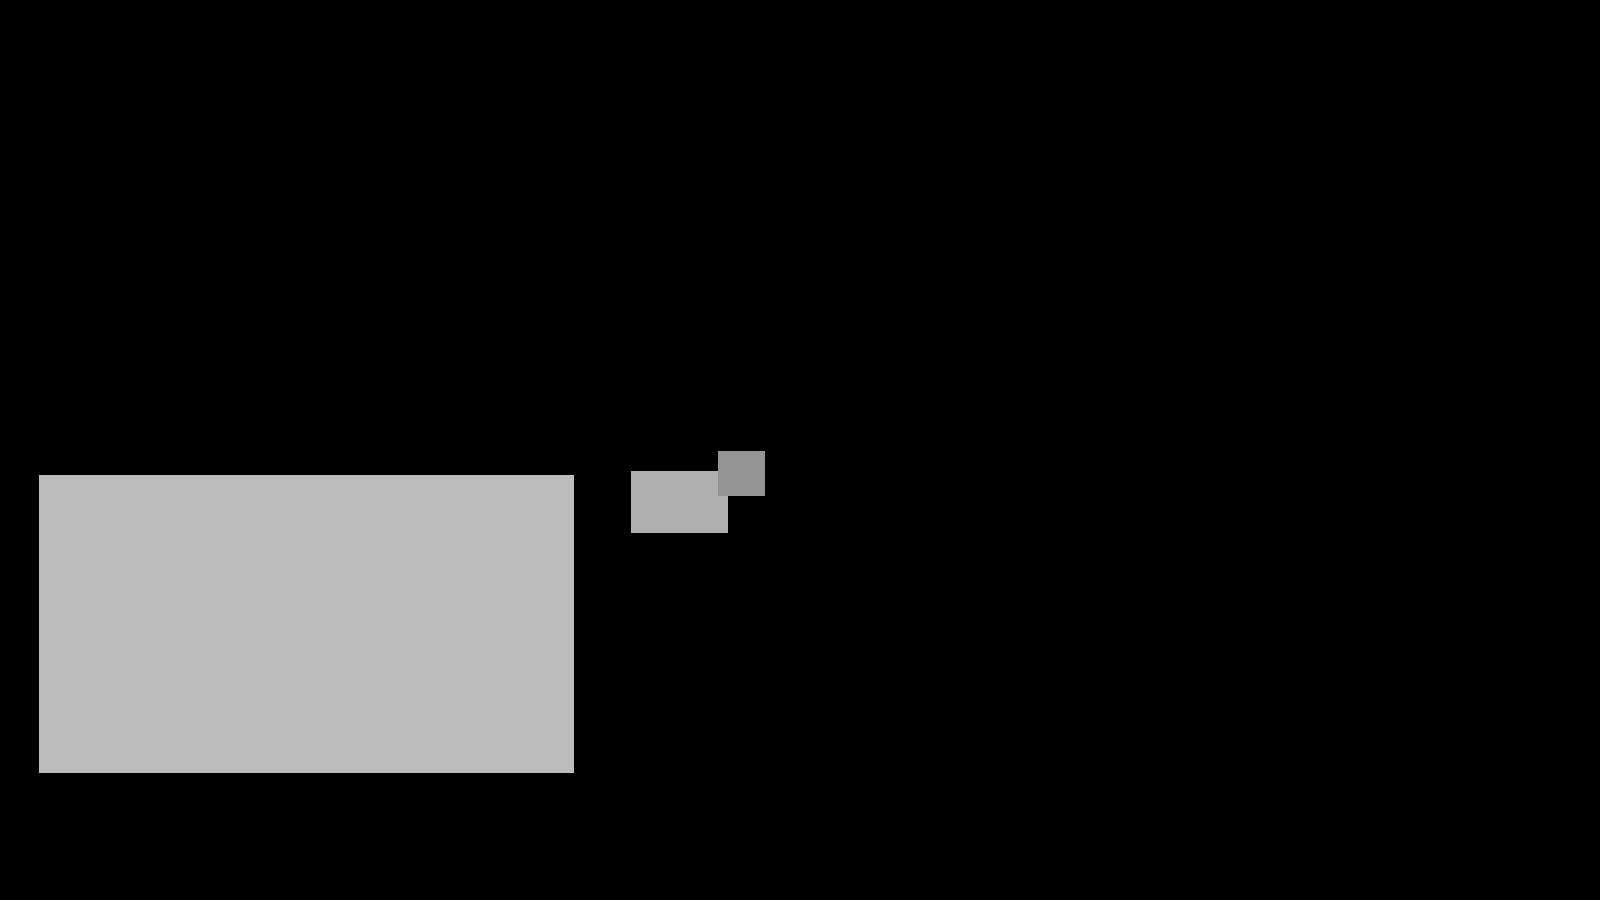}
    \end{minipage}
    \begin{minipage}{0.35\textwidth}
        \centering
        \includegraphics[height=2.7cm]{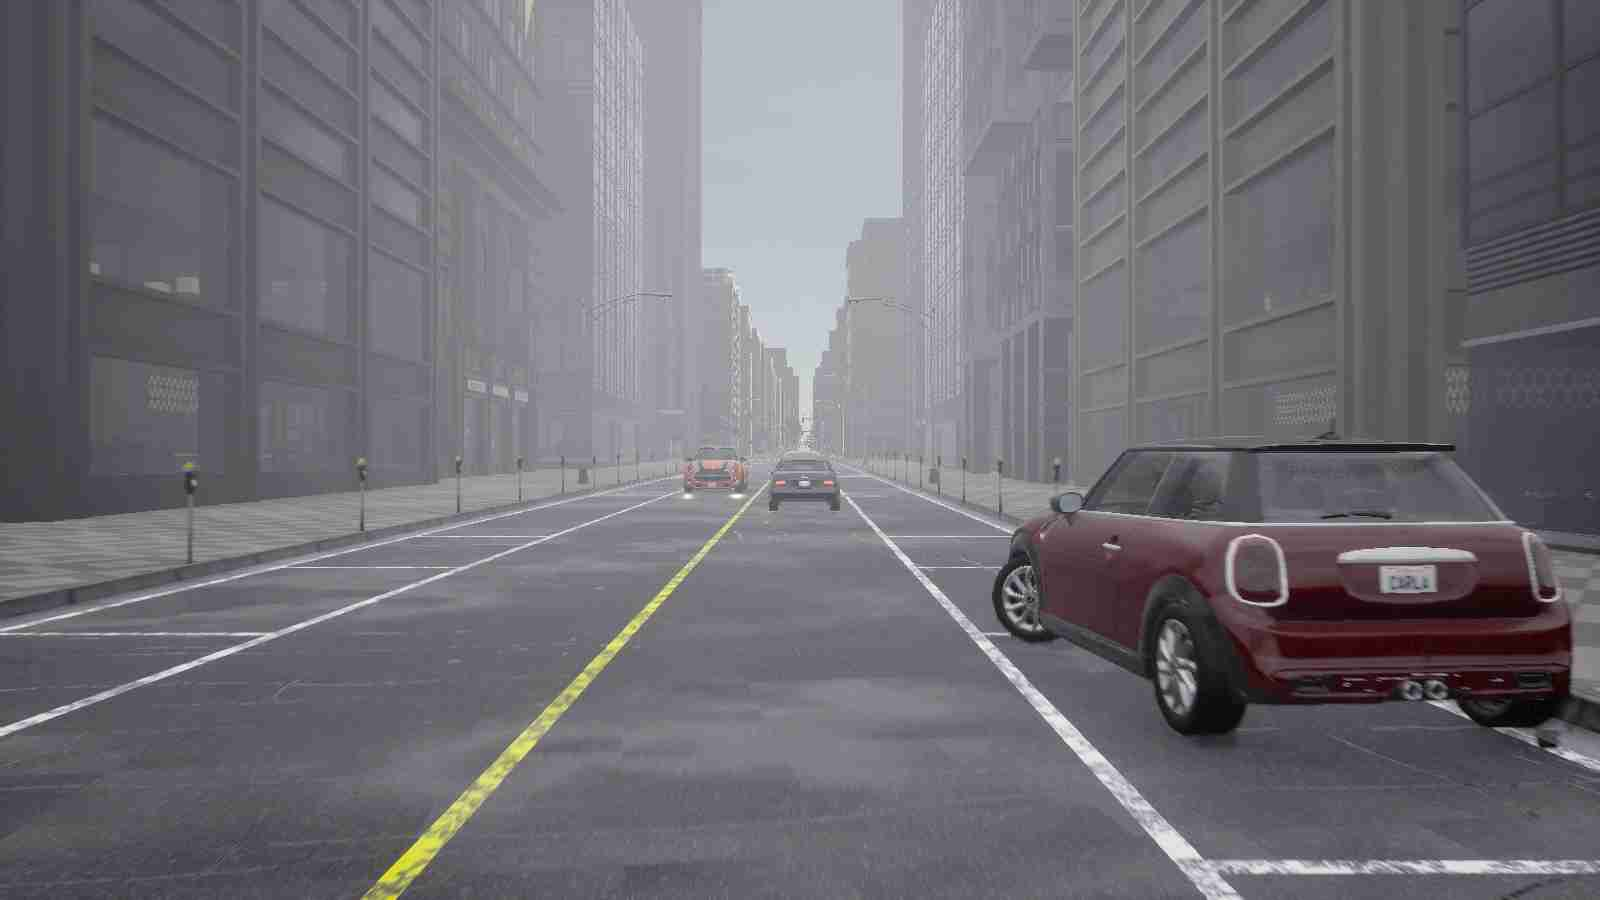}
    \end{minipage}
    \begin{minipage}{0.35\textwidth}
        \centering
        \includegraphics[height=2.7cm]{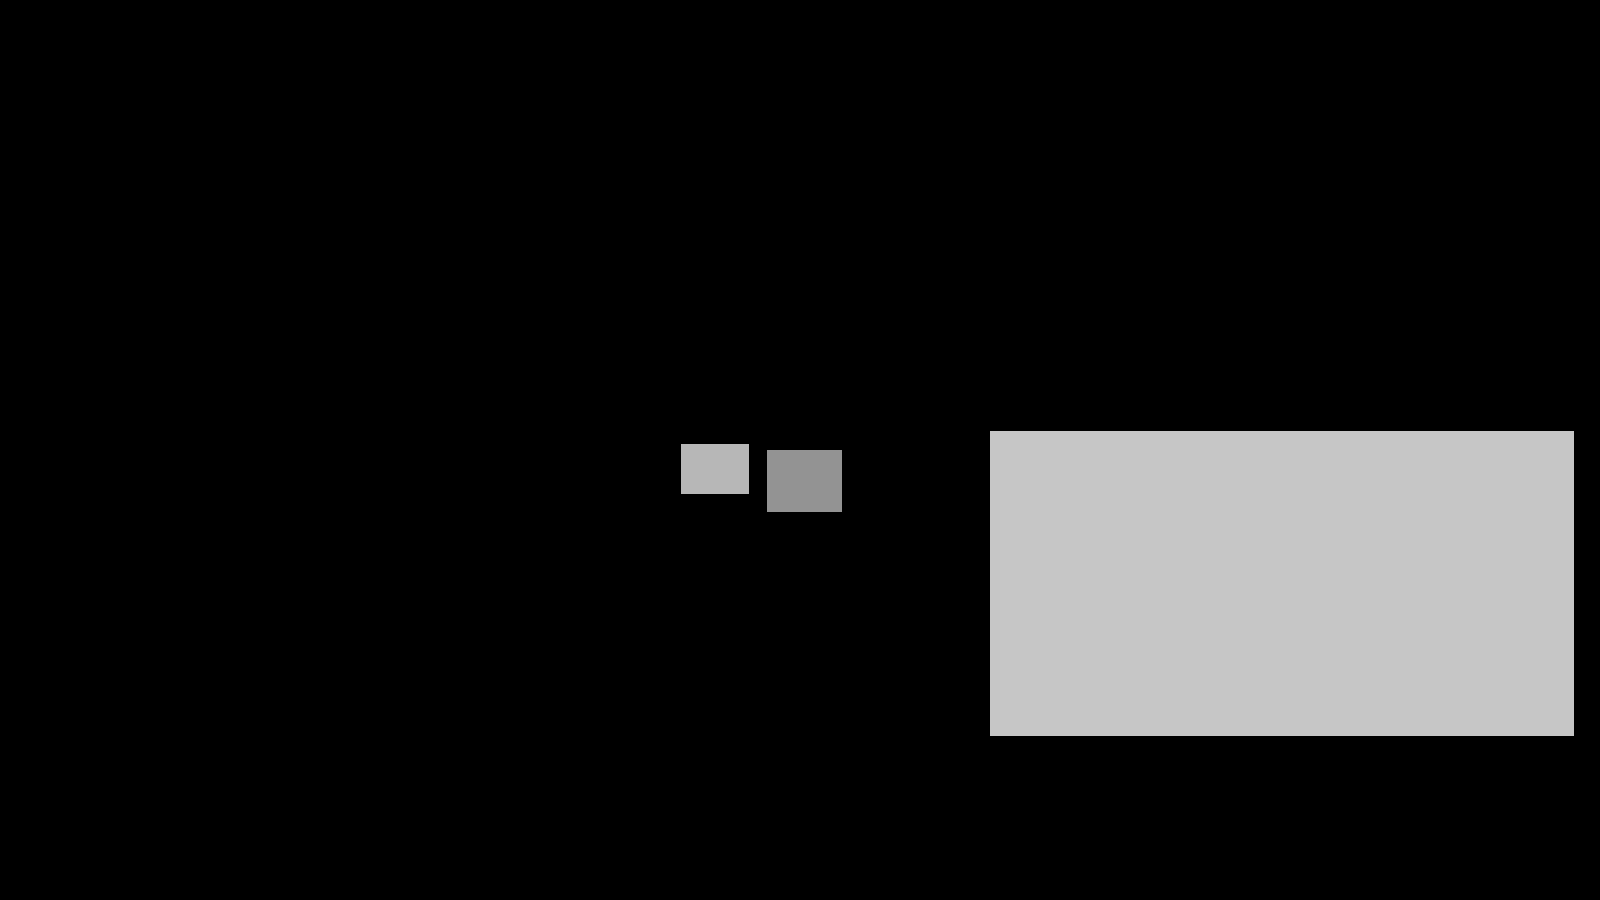}
    \end{minipage}
    \begin{minipage}{0.35\textwidth}
        \centering
        \includegraphics[height=2.7cm]{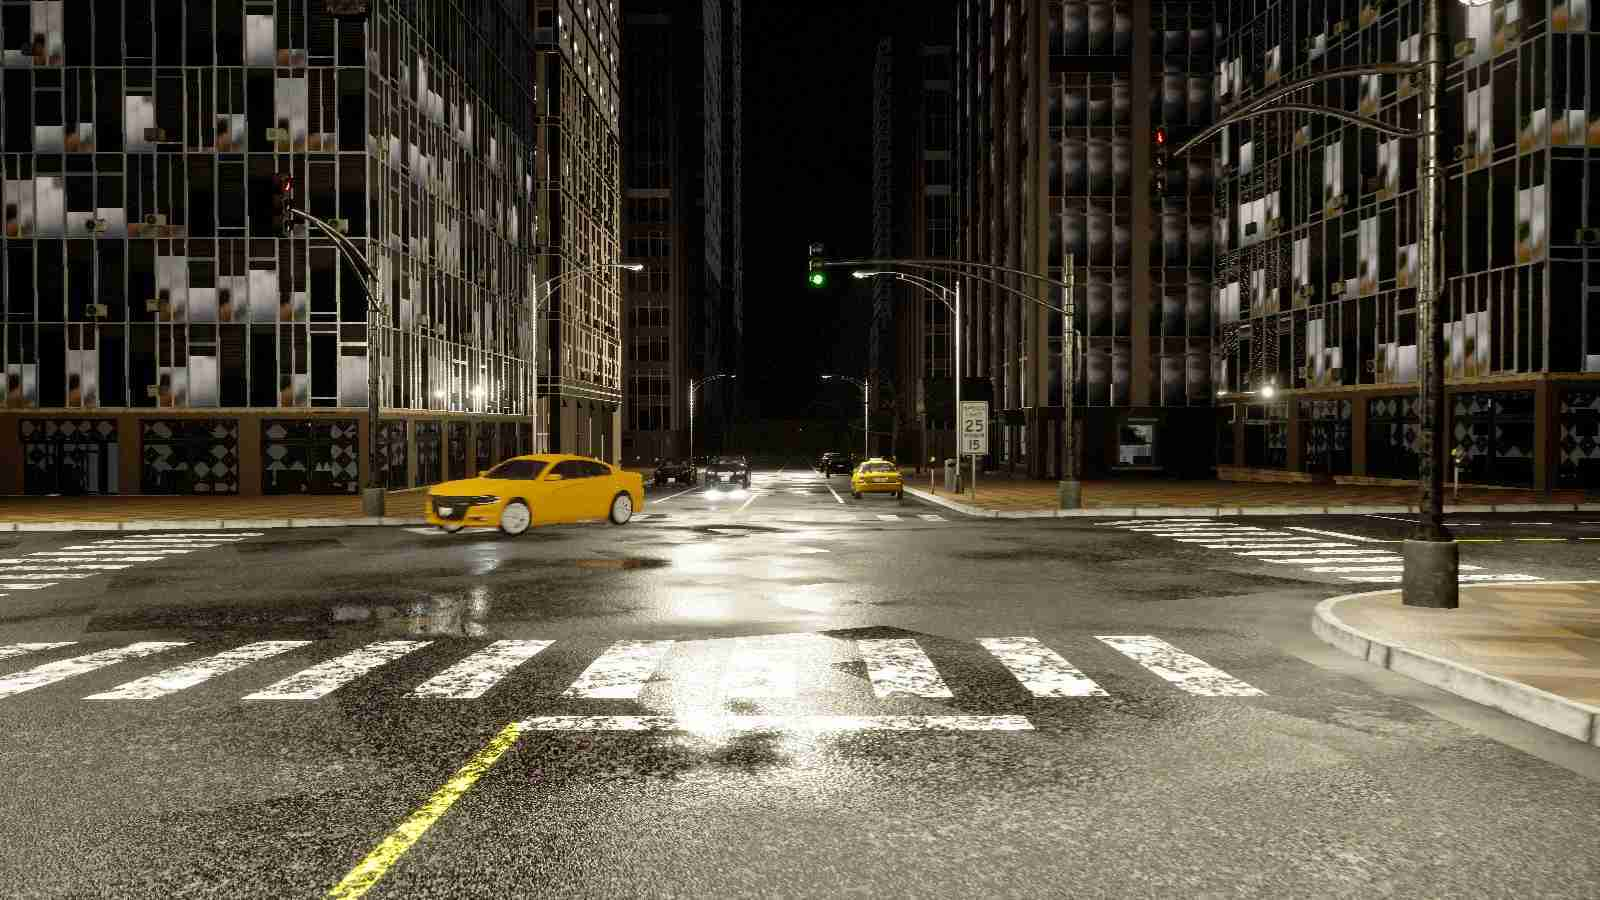}
    \end{minipage}
    \begin{minipage}{0.35\textwidth}
        \centering
        \includegraphics[height=2.7cm]{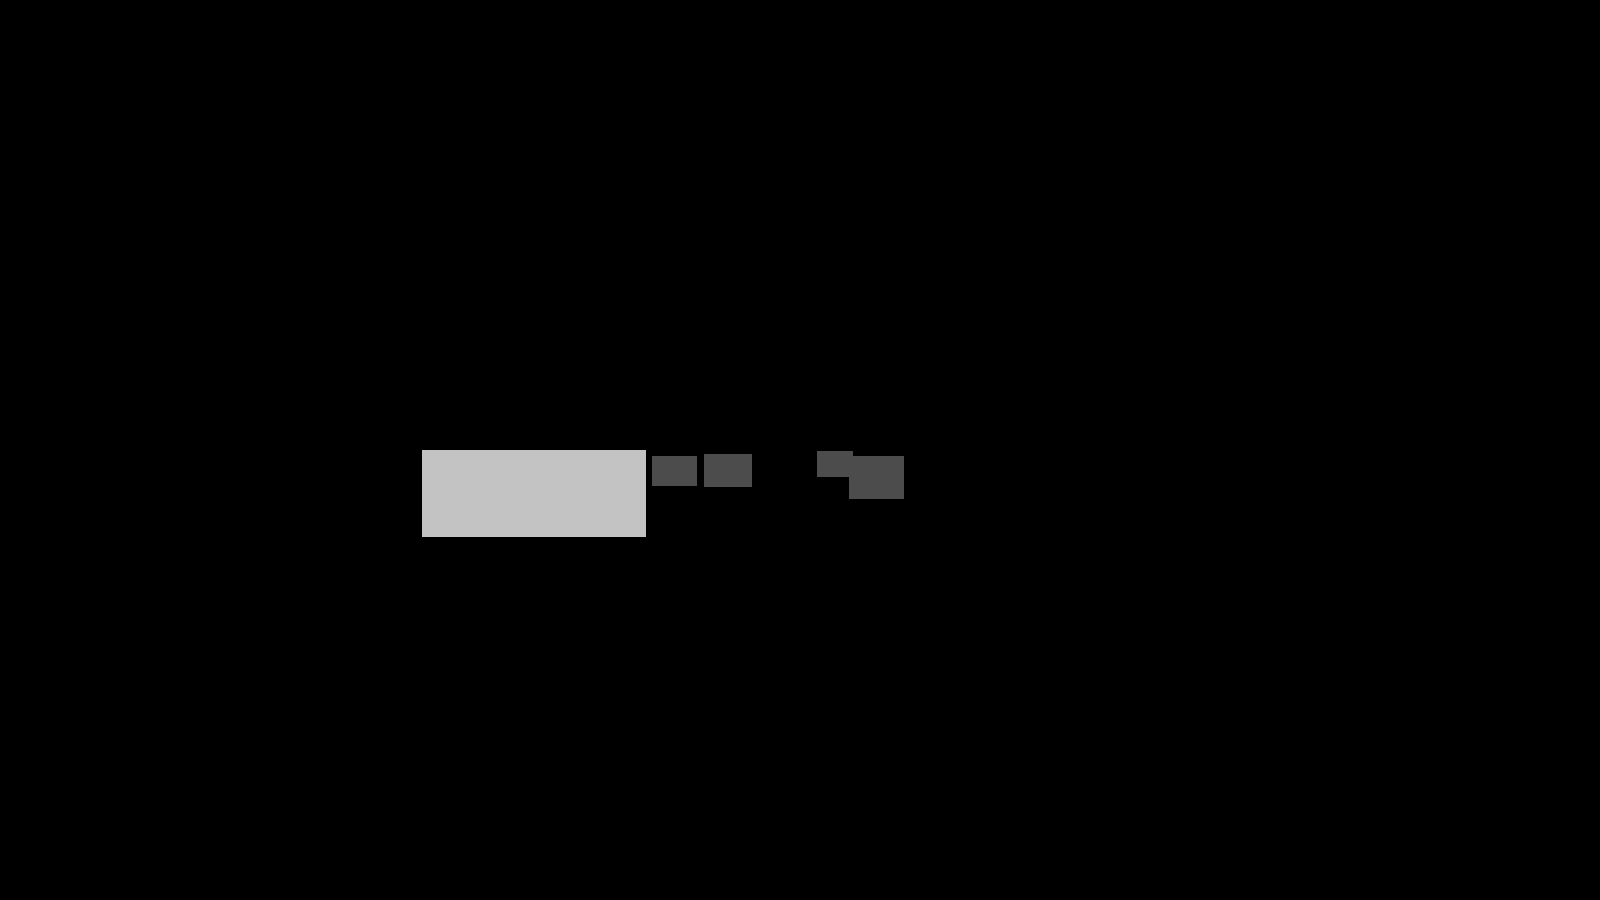}
    \end{minipage}
    \caption{\textbf{Risk Head Reconstruction}. Visualization of Risk Object Localization using Bounding Boxes. This figure illustrates the effectiveness of the risk prediction head in localizing risk objects through coarse-grained bounding box supervision. Each row presents a real-world urban driving scene (left) alongside the corresponding risk prediction mask generated by the model (right), where high-risk objects are highlighted.}
    \label{fig:Bbox-RSD}
\end{figure*}
As shown in Fig.~\ref{fig:Bbox-RSD}. By leveraging simple bounding boxes instead of dense pixel-level annotations, our approach significantly reduces the annotation cost and training complexity, while still enabling the model to focus on semantically meaningful, high-risk regions. The visualized results show that the risk head consistently attends to critical objects (e.g., crossing vehicles, occluded cars, or oncoming traffic), validating its ability to extract interpretable and task-relevant risk semantics. This demonstrates that the bounding box–based risk estimation offers an efficient and scalable solution for risk-aware perception in autonomous driving.

\subsection{RSD Results}
\label{RSD Results}
\begin{figure*}[htbp]
    \centering
    % 左侧的单独大图
    \begin{minipage}{0.35\textwidth}
        \centering
        \includegraphics[height=2.7cm]{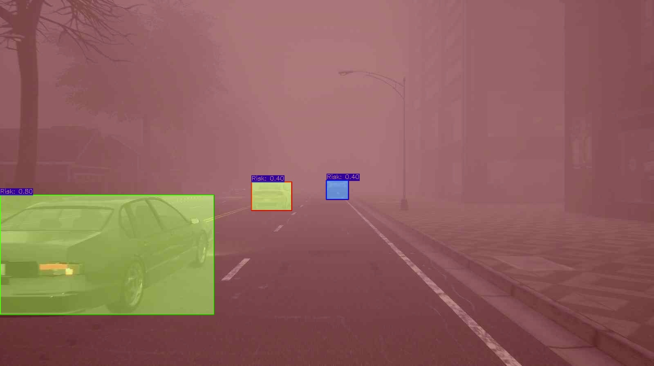}
    \end{minipage}
    \begin{minipage}{0.35\textwidth}
        \centering
        \includegraphics[height=2.7cm]{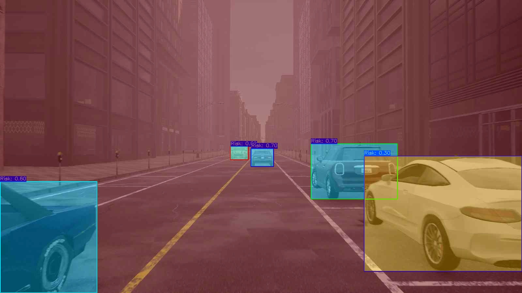}
    \end{minipage}
    \begin{minipage}{0.35\textwidth}
        \centering
        \includegraphics[height=2.7cm]{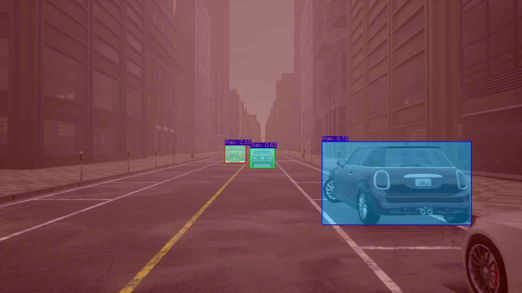}
    \end{minipage}
    \begin{minipage}{0.35\textwidth}
        \centering
        \includegraphics[height=2.7cm]{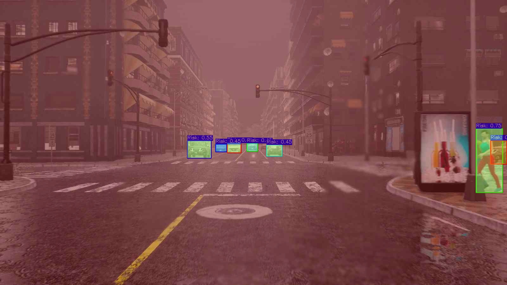}
    \end{minipage}
    \begin{minipage}{0.35\textwidth}
        \centering
        \includegraphics[height=2.7cm]{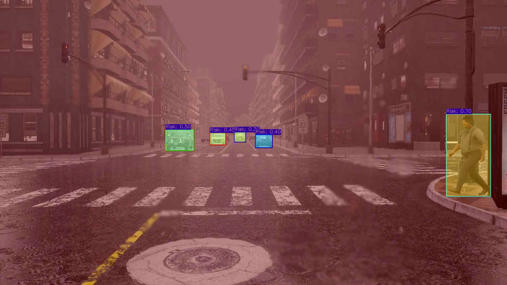}
    \end{minipage}
    \begin{minipage}{0.35\textwidth}
        \centering
        \includegraphics[height=2.7cm]{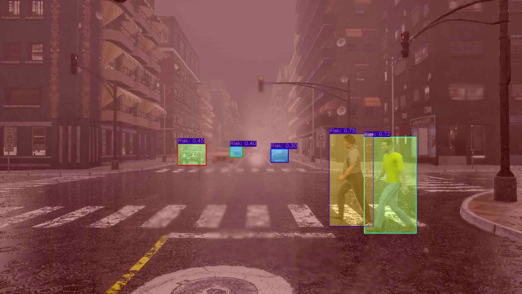}
    \end{minipage}
    \begin{minipage}{0.35\textwidth}
        \centering
        \includegraphics[height=2.7cm]{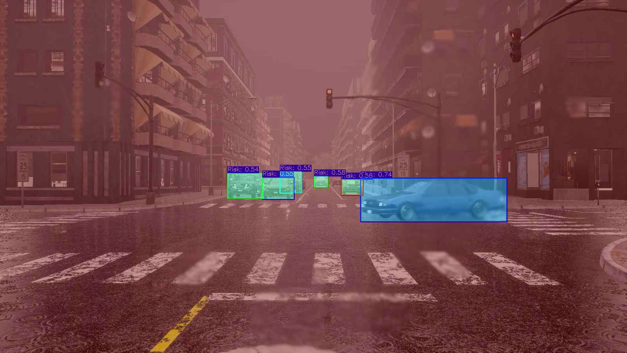}
    \end{minipage}
    \begin{minipage}{0.35\textwidth}
        \centering
        \includegraphics[height=2.7cm]{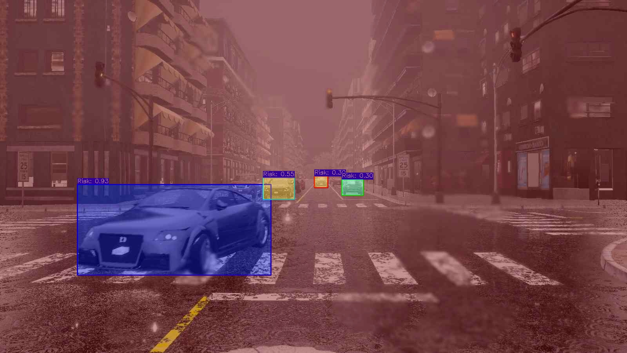}
    \end{minipage}
    \begin{minipage}{0.35\textwidth}
        \centering
        \includegraphics[height=2.7cm]{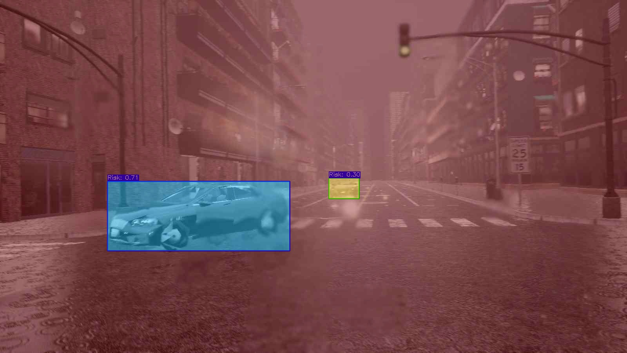}
    \end{minipage}
    \begin{minipage}{0.35\textwidth}
        \centering
        \includegraphics[height=2.7cm]{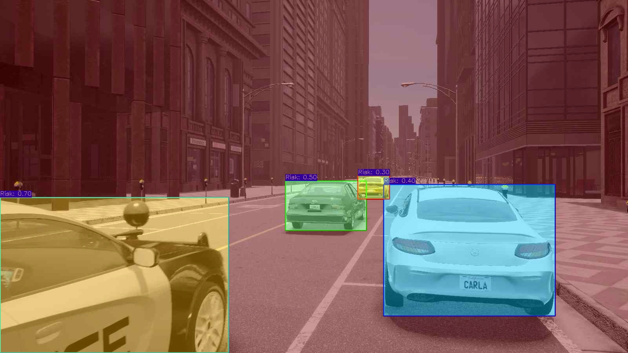}
    \end{minipage}
    \caption{\textbf{Risk Head Reconstruction}. This figure presents qualitative results from the risk prediction head demonstrating its ability to reconstruct risk semantics from the BEV representation. In each image, the highlighted bounding boxes indicate the model's estimation of critical risk objects including vehicles, pedestrians, and other road users.}
    \label{fig:RSD-Results}
\end{figure*}

As shown in Fig.~\ref{fig:RSD-Results}. The varying colors reflect different object categories and inferred risk levels. Notably, the model consistently focuses on semantically important regions—such as occluded or oncoming vehicles pedestrians near crosswalks and objects in the vehicle's intended path—even under challenging visual conditions (e.g., low visibility or dense traffic). These visualizations confirm that the risk head effectively learns to identify and prioritize high-risk entities, offering interpretable and context-aware predictions. This supports the claim that RSD enables the driving model to attend to safety-critical cues without the need for dense annotations or external risk supervision.
\section{Conclusion and Limitations}
\label{Conclusion and Limitations}
The Risk Semantic Distillation (RSD) framework offers several notable advantages:

1. Strong Inference Efficiency: Unlike other Vision-Language Model (VLM) based Autonomous Driving (AD) architectures, RSD directly distills the capabilities of large models into the AD backbone network. This results in highly efficient inference, which is crucial for real-time decision-making in autonomous driving systems.

2. Scalability and Mass Production Potential: Due to its efficient design, RSD has strong potential for large-scale deployment in the autonomous driving industry. The ability to distill the power of large models into a compact and efficient architecture makes it feasible for mass production, meeting the operational demands of real-world applications.

3. Effective Integration of VLM Capabilities: By directly incorporating the advanced capabilities of large pre-trained VLMs into the AD system, RSD enhances object detection and risk semantic annotation, making the system better at identifying and prioritizing critical risk objects in complex environments.

4. Real-World Application Potential: The framework's design emphasizes practical application in the autonomous driving domain, where it can be applied to a variety of driving scenarios. Its capacity for real-time, efficient processing and scalable deployment makes it highly suitable for large-scale adoption.

In summary, RSD stands out for its high inference efficiency, scalability, and real-world applicability, making it a promising solution for advancing autonomous driving systems.

\subsection{Limitations}
\label{Limitations}
Future work is needed to further investigate and improve the quality of risk semantic annotation, particularly in terms of consistency, granularity, and alignment with real-world driving risk factors. Enhanced benchmarks, annotation protocols, and evaluation metrics will be essential to ensure reliable supervision signals and to support the development of more robust and generalizable autonomous driving models.

\newpage
\section{Experiments compute resources}
\label{Experiments compute resources}
%The inference latency of VAD-Tiny is measured on a single NVIDIA GeForce RTX 3090 GPU and remains under 60ms. 
The model is lightweight, with a total parameter size of approximately 50M. The model's weight size is approximately 1\% of that of typical VLM-AD architectures, resulting in over a 10× improvement in inference efficiency. This lightweight design enables real-time deployment while retaining the essential risk-aware capabilities distilled from large-scale vision-language models. This low-latency and compact design makes VAD-Tiny well-suited for real-time autonomous driving applications.
\vspace{-15pt}
\subsection{Code and Video}
\label{Code and Video}
All code and videos are available in \url{https://anonymous.4open.science/r/RSD-3FCE}.

\section{Closed-loop Experiment}

\subsection{Experimental Settings}
In our closed-loop simulation experiment within the CARLA environment, we trained our model using only a \textbf{tiny subset} of the Bench2Drive dataset—specifically, \textbf{10\%} of the base dataset and \textbf{1\%} of the full dataset. For validation, we employed the \textbf{Dev10 benchmark}\cite{jia2024bench2drive,jia2025drivetransformer}, comprising 10 carefully selected clips from the official 220 routes. These clips were chosen to be both challenging and representative, exhibiting low variance, which is officially recommended for ablation studies to prevent overfitting on the entire Bench2Drive220 routes. The details can be found in Tab.~\ref{tab:dev10_routes}. 

\begin{table}[ht]
\centering
\caption{Routes of Dev10 protocol.}
\label{tab:dev10_routes}
\begin{tabular}{lccc}
\toprule
\textbf{Scenario} & \textbf{Route-ID} & \textbf{Road-ID} & \textbf{Town} \\
\hline
ParkingExit & 3514 & 892 & 13 \\
ParkingCrossingPedestrian & 3255 & 1237 & 13 \\
StaticCutIn & 26405 & 137 & 15 \\
HazardAtSideLane & 25381 & 37 & 05 \\
YieldToEmergencyVehicle & 25378 & - & 03 \\
ConstructionObstacleTwoWays & 25424 & 269 & 11 \\
NonSignalizedJunctionLeftTurn & 2091 & - & 12 \\
BlockedIntersection & 27494 & 16 & 04 \\
SequentialLaneChange & 16569 & 1157 & 12 \\
SignalizedJunctionLeftTurnEnterFlow & 28198 & 234 & 15 \\
\bottomrule
\end{tabular}
\end{table}

\subsection{Closed-loop Metric}
As shown in Tab.~\ref{tab:Closed-Loop Experiment}, the results demonstrate that integrating the RSD plugin into End-to-End backbone significantly enhances the performance of the VAD model.

\begin{table*}[ht]
\centering
\caption{Closed-Loop Experiment.}
\begin{tabular}{ccccccc}
\toprule
Method & Driving Score$\uparrow$ & Success Rate$\uparrow$\\
\midrule
VAD-Tiny &36.306 & 0.167\\
\textbf{VAD-Tiny-RSD} & \textbf{46.662} & \textbf{0.278} \\
% \textbf{Flying Dog Real(ours)} & \textbf{Unitree-Go1} & \textbf{2.2} & \textbf{2.5} & \textbf{45$^{\circ}$} & \textbf{\checkmark} \\
\bottomrule
\end{tabular}
\label{tab:Closed-Loop Experiment}
\end{table*}

% \subsection{Experiments Compute Resources}
% \label{Experiments Compute Resources}
% Owing to the modular plug-in design of RSD, the inference latency of VAD-Tiny-RSD remains unchanged compared to that of the baseline VAD-Tiny model. The inference latency of VAD-Tiny is measured on a single NVIDIA GeForce RTX 3090 GPU and remains under 60ms. The model is lightweight, with a total parameter size of approximately \textbf{50M}. The model's weight size is approximately \textbf{1\%} of that of typical VLM-AD architectures, resulting in resulting in \textbf{a more than tenfold improvement} in inference efficiency. This lightweight design enables real-time deployment while retaining the essential risk-aware capabilities distilled from large-scale vision-language models. The low-latency and compact design makes VAD-Tiny well-suited for real-time autonomous driving applications.

% \subsection{Code and Video}
% \label{Code and Video}
% All code and videos are available in \url{https://anonymous.4open.science/r/RSD-3FCE}.
